# Supplementary material for: Strain-engineered inverse charge-funnelling in layered semiconductors
Source: arXiv:1801.09434 ancillary file (2018-01-29)
Supplement: Supplementary file 1 [file SUPPLEMENTARY_paper_HfS2_AdeS.pdf]

# SUPPLEMENTARY MATERIAL

## Strain-engineered inverse charge-funnelling in layered semiconductors

Adolfo De Sanctis, Iddo Amit, Steven P. Hepplestone, Monica F. Craciun, and  
Saverio Russo\*

*Centre for Graphene Science, College of Engineering, Mathematics and Physical Sciences,  
University of Exeter, Exeter EX4 4QF, United Kingdom*

E-mail: S.Russo@exeter.ac.uk

### Contents

|                                                                                  |           |
|----------------------------------------------------------------------------------|-----------|
| <b>S1 Photo-oxidation mechanism</b>                                              | <b>3</b>  |
| <b>S2 Supplementary AFM and spectroscopy data</b>                                | <b>5</b>  |
| S2.1 Laser-induced oxidation: AFM data . . . . .                                 | 5         |
| S2.2 Photon assisted oxidation of bulk HfS <sub>2</sub> . . . . .                | 7         |
| S2.3 Supplementary AFM data . . . . .                                            | 8         |
| S2.4 Visible wavelength absorption and photoluminescence extended data . . . . . | 9         |
| <b>S3 First principles calculations</b>                                          | <b>10</b> |
| S3.1 Reactions energy cost . . . . .                                             | 10        |
| S3.2 HfS <sub>2</sub> and HfO <sub>2</sub> band structure . . . . .              | 11        |

---

\*To whom correspondence should be addressed

|                                                                              |           |
|------------------------------------------------------------------------------|-----------|
| <b>S4 Supplementary photoresponse data</b>                                   | <b>12</b> |
| S4.1 Electrical characterization . . . . .                                   | 12        |
| S4.2 Extended photocurrent mapping data . . . . .                            | 12        |
| <b>S5 Analytical model describing the observed SPCM response</b>             | <b>14</b> |
| <b>S6 Supplementary discussion on PV enhancement using charge funnelling</b> | <b>18</b> |

# S1 Photo-oxidation mechanism

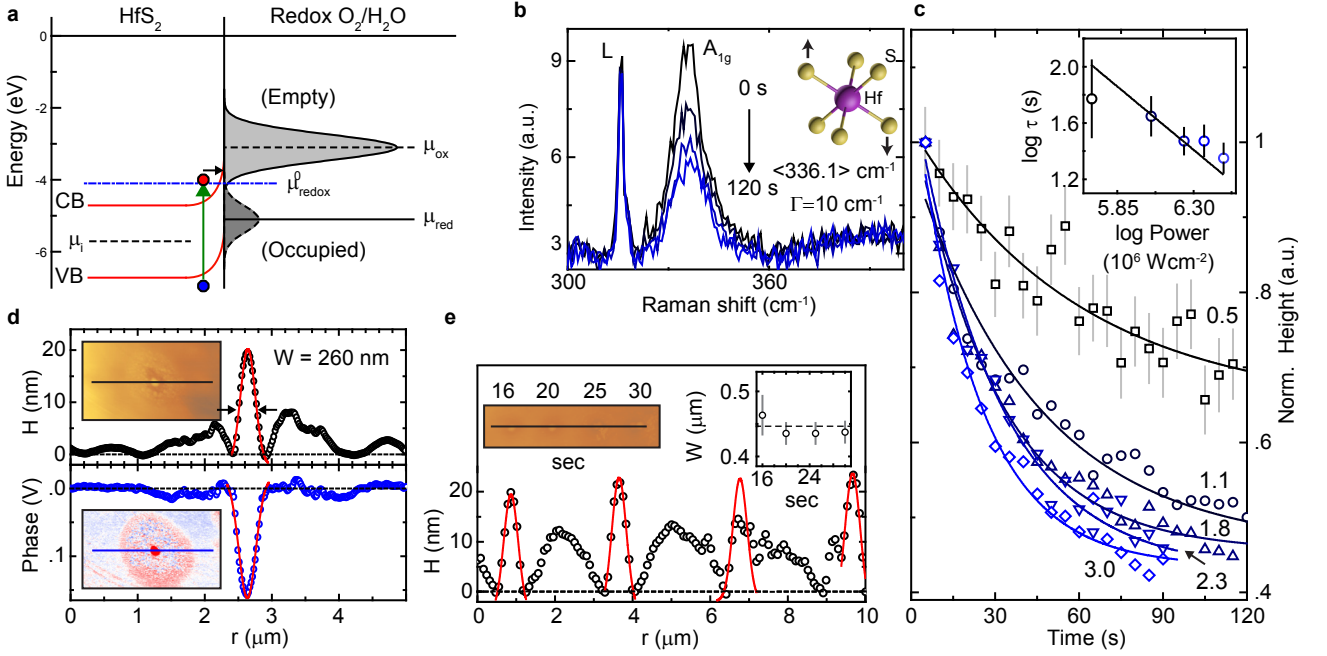

Figure S1: **Charge-Transfer model and photo-oxidation of HfS<sub>2</sub>.** **a**, Schematic energy diagram of multi-layer HfS<sub>2</sub> in contact with the redox couple O<sub>2</sub>/H<sub>2</sub>O present in air in atmospheric conditions.<sup>1</sup> The chemical potentials of the oxidizing and reducing species are  $\mu_{ox} = -3.1$  eV and  $\mu_{ox} = -5.1$  eV, respectively. The chemical potential of the oxygen acceptor state is  $\mu_{redox}^0 = -4.1$  eV. The intrinsic work function of HfS<sub>2</sub> is  $\mu_i = -5.7$  eV with  $E_g = 1.96$  eV. **b**, Time evolution of the HfS<sub>2</sub> A<sub>1g</sub> Raman mode at  $336.1 \pm 0.01$  cm<sup>-1</sup> (average), with FWHM 10 cm<sup>-1</sup>, upon laser exposure ( $\lambda = 514$  nm,  $P = 3.0$  MW/cm<sup>2</sup>) of a 4.9 nm thick flake. The peak named L corresponds to a spurious laser line (note no change of this line in the spectra). **c**, Normalized A<sub>1g</sub> mode height as a function of time for different incident laser powers (0.5 - 3.0 MW/cm<sup>2</sup>), solid lines mark monoexponential decays; Inset: log-log plot of decay time  $\tau$  versus incident power density, solid line marks a slope of -1. **d**, AFM topography (top) and phase signal (bottom) of a 80 nm-thick laser-irradiated flake ( $\lambda = 375$  nm,  $P = 1.5$  MW/cm<sup>2</sup>, 10 seconds exposure), a Gaussian peak can be fitted with a FWHM of 260 nm. **e**, AFM topography of the same flake with laser-irradiated spots for different exposure times ( $\lambda = 473$  nm,  $P = 4.3$  MW/cm<sup>2</sup>). Inset: FWHM of the Gaussian fits as a function of exposure time, dashed line marks the average value of 446 nm.

Following the model in ref. 2, we propose in figure S1a the energy diagram of the interface between HfS<sub>2</sub> and aqueous oxygen in atmosphere<sup>1</sup> provided by the reaction  $2H_2O \rightleftharpoons O_2(aq) + 4e^- + 4H^+$ . The intrinsic chemical potential of HfS<sub>2</sub> is  $\mu_i = -5.2$  eV (calculated from the distance from the vacuum level to the top of the valence band,  $\phi = -6.68$  eV and

indirect bandgap  $E_g = 1.96$  eV), while that of the oxygen acceptor state is  $\mu_{\text{redox}}^0 = -4.1$  eV. This induces a band-bending at the surface of the layered semiconductor such that an optical transition above the bandgap can make an electron ready to be transferred to the oxygen empty states, making the photo-oxidation reaction highly feasible across the whole visible range, explaining the high instability of few-layer  $\text{HfS}_2$  in atmospheric conditions. The CT reaction starts with a photon of energy  $h\nu$  impinging on  $\text{HfS}_2$ , which produces an optical excitation, leaving the material in an excited state:  $\text{HfS}_2 + h\nu \longrightarrow \text{HfS}_2^*$ . This state provides the carriers for the CT reaction at the surface according to the following:

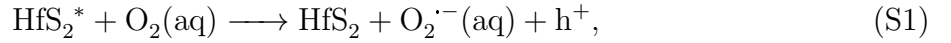

the oxygen radical ion  $\text{O}_2^{\cdot-}(\text{aq})$  can then react with the  $\text{HfS}_2$  and, upon cleavage of the Hf–S bond, bind to the Hf and S, respectively:

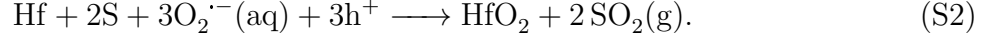

Therefore the total reaction can be written as:

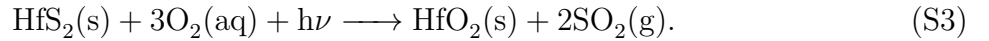

Marcus-Gerischer theory (MGT)<sup>1</sup> gives an estimation of the rate of change in the pristine material composition:

$$\frac{d\Theta}{dt} \propto \Theta \Phi_{ph} [\text{O}_2] \exp \left[ -\frac{\left( \frac{E_g}{2} + E_i - E_{\text{F,red}}^0 - \lambda \right)^2}{4k_b T \lambda} \right], \quad (\text{S4})$$

where  $\Theta$  is the amount of pristine material,  $\Phi_{ph}$  is the laser flux,  $[\text{O}_2]$  is the oxygen concentration,  $E_g$  is the direct gap energy,  $E_i$  is the intrinsic Fermi level,  $E_{\text{F,red}}^0$  is the energy of the oxygen acceptor state ( $\sim 3.1$  eV) with respect to the vacuum level,  $\lambda$  is the renormalization energy of oxygen in water ( $\sim 1$  eV),  $k_b$  is the Boltzmann constant and  $T$  the temperature.<sup>1</sup>

Therefore, the oxidation rate depends on the laser flux  $\Phi_{ph}$  and the initial amount of pristine material  $\Theta_0$ :  $\Theta \propto \Theta_0 \exp(-t/\tau)$  where the decay time  $\tau \propto \Phi_{ph}^{-1}$ . This dependence is experimentally verified in figure S1b-c where the intensity of the Raman  $A_{1g}$  mode of  $\text{HfS}_2$ , an indication of the amount of pristine material present in the sampling volume, is plotted against time for different laser fluxes. Monoexponential decay fits give a decay time  $\tau$  with the expected power relation (figure S1c, inset).

Figure figure S1d shows that the oxidized area is compatible with the diffraction-limited spot size of our laser system (see methods). Indeed, the AFM topography and tapping phase images of an exposed thick (80 nm) flake shows a bubble-like structure with a 25 % increase in height. This feature shows a Gaussian profile with a full-width at half-maximum (FWHM) of 260 nm. We then exposed different areas of the flake, for different lengths of time while keeping the laser power density constant. As shown in figure S1e, no changes in the FWHM of the Gaussian profile is observed. All these observations confirm that photon-assisted oxidation is taking place, as opposed to thermal oxidation.

## S2 Supplementary AFM and spectroscopy data

### S2.1 Laser-induced oxidation: AFM data

In figure S2 we report additional data on the laser-induced oxidation process in  $\text{HfS}_2$ . Figure S2a-d show the AFM data acquired on a flake with different layers deposited on a  $\text{Si}/\text{SiO}_2$  substrate (oxide thickness 285 nm). Different areas of the flake were exposed with  $\lambda_{\text{exc}} = 532$  nm at a power of  $0.1 \text{ MW}/\text{cm}^2$  for 20 s, using a commercial *Renishaw* micro-Raman spectroscopy system. A marked change of contrast in the areas of  $\text{HfS}_2$  exposed to the laser is visible in the white light optical micrograph (see figure S2a). Though the observed change of contrast might suggest that  $\text{HfS}_2$  has been ablated by the laser, a detailed study of the topography of the flakes with atomic force microscopy demonstrates that this is not the case, see figure S2b. Indeed, we measured that the average height of the laser-exposed area is the

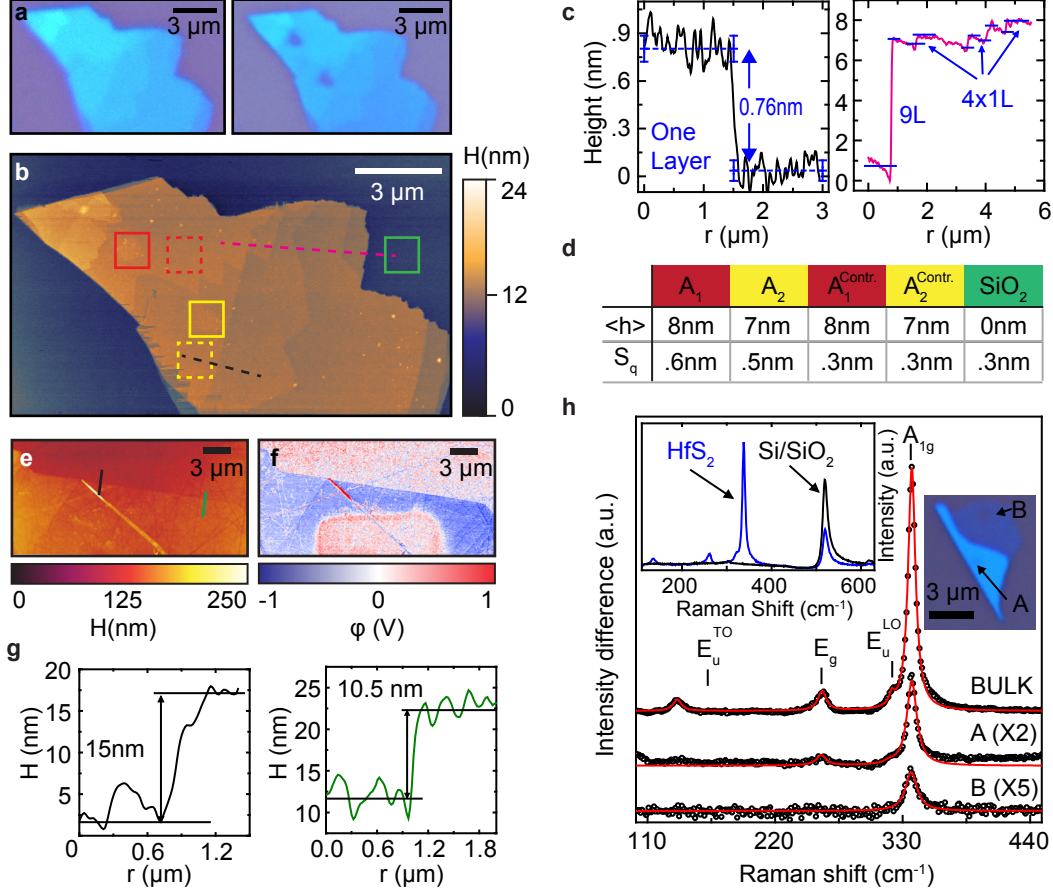

Figure S2: **Supplementary AFM data on laser-induced oxidation.** **a**, Optical micrographs of an HfS<sub>2</sub> flake before (left) and after (right) exposure of two areas with  $\lambda_{\text{exc}} = 532$  nm at 0.1 MW/cm<sup>2</sup> incident power for 20 s. **b**, AFM topography of the same flake shown in **a**. The straight dashed lines correspond to the regions for profiles shown in panel **c**, where the height of a single layer is measured to be  $0.76 \pm 0.08$  nm. Solid squares enclose the laser-exposed regions, dashed squares enclose the control regions used for statistical analysis. **d**, Statistical analysis of AFM topography shown in **b**:  $\langle h \rangle$  is the average height measured in the square and  $S_q$  is the RMS surface roughness. **e**, AFM topography and **f** tapping phase images of the HfS<sub>2</sub> flake presented in Figure 1a main text, after laser exposure of the central area. **g**, Height profiles across the solid lines shown in **e**. **h**, Raman spectra of HfS<sub>2</sub> acquired on a bulk sample ( $> 100 \mu\text{m}$  thick) and on a thinner flake exfoliated on Si/SiO<sub>2</sub> (areas A and B in the optical micrograph), after subtraction of the pristine substrate spectrum (inset).

same as the nearby control area (figure S2d),  $\langle h \rangle \simeq 8$  nm, while the RMS height of the surface (roughness),  $S_q$ , is increased by  $\sim 50\%$  with respect to the control areas (which have an  $S_q$  value comparable with that of the underlying substrate).

Figure S2e-g show additional AFM data for the flake of figure 1 in the main text. The AFM topography and tapping phase images are shown in panels e and f, respectively. Panel g shows the height profiles for the two different regions of the flake. The height of one layer of  $\text{HfS}_2$  was measured to be  $0.76 \pm 0.08$  nm (panel c), thus the aforementioned flake has a thickness of  $\sim 20$  and  $\sim 14$  layers in the two regions across which the laser was scanned.

In figure S2h we report the Raman spectra of  $\text{HfS}_2$  on a  $\text{Si}/\text{SiO}_2$  substrate, shown in the optical micrograph inset. In the bulk material we observe all the first order Raman modes:  $A_{1g} = 337$   $\text{cm}^{-1}$ ,  $E_g = 260$   $\text{cm}^{-1}$ ,  $E_u(\text{LO}) = 321$   $\text{cm}^{-1}$  and  $E_u(\text{TO}) = 136$   $\text{cm}^{-1}$ ; All these modes are well described by a fit with a Lorentzian curve with a FWHM  $\sim 10$   $\text{cm}^{-1}$  and the peak positions agree well with previous studies,<sup>3-5</sup> except for the  $E_u(\text{TO})$  mode which appears blue-shifted (literature value  $\sim 155 - 166$   $\text{cm}^{-1}$ ). For thinner flakes we observe that it is increasingly difficult to acquire a spectrum as the material is thinned. To the best of our knowledge no reports have shown the isolation of single-layer  $\text{HfS}_2$ .

## S2.2 Photon assisted oxidation of bulk $\text{HfS}_2$

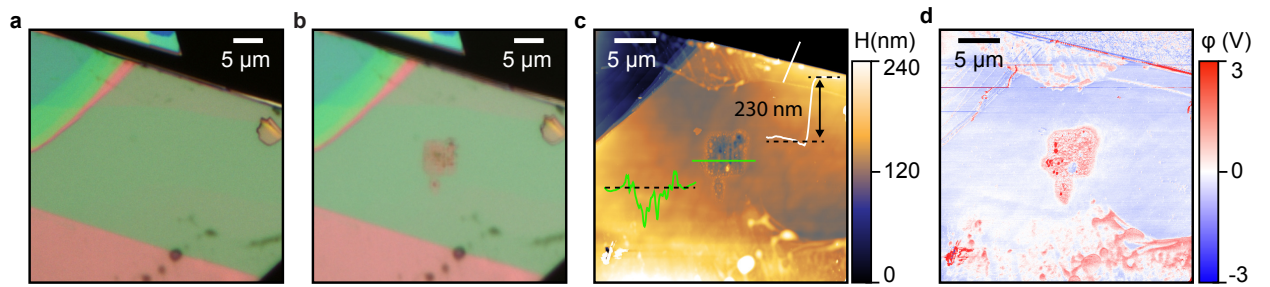

Figure S3: **Thick flakes photo-oxidation and damage.** **a-b**, Optical micrograph of a thick flake before (**a**) and after (**b**) laser exposure of a  $5 \times 5$   $\mu\text{m}$  square, with  $\lambda_{\text{exc}} = 375$  nm ( $P = 5.0$   $\text{MW}/\text{cm}^2$ ), scanned in steps of  $0.5$   $\mu\text{m}$ , exposing each point for  $20$  s. **c-d**, AFM topography (**c**) and tapping phase (**d**) images of the flake shown in **a**. Insets show the thickness of the flake (white),  $\delta = 230$  nm, and the height profile of the laser exposed area (green), the black dotted line marks the average height of the pristine flake.

Figure S3 shows the photo-oxidation of a thick (230 nm)  $\text{HfS}_2$  flake. A comparison of micrograph pictures before (figure S3a) and after (figure S3b) exposing with a laser a  $5 \times 5 \mu\text{m}$  square area ( $\lambda_{\text{exc}} = 375 \text{ nm}$ ,  $P = 5.0 \text{ MW}/\text{cm}^2$ ,  $0.5 \mu\text{m}$  steps each exposed for 20 s) shows that for bulk flakes the oxidation does not involve the whole thickness, as it is not possible to see the substrate underneath the flake. Indeed, AFM topography (figure S3c) and tapping phase (figure S3d) show that the surface of the flake is damaged after prolonged exposure, as shown by the line profiles across the laser-exposed region.

### S2.3 Supplementary AFM data

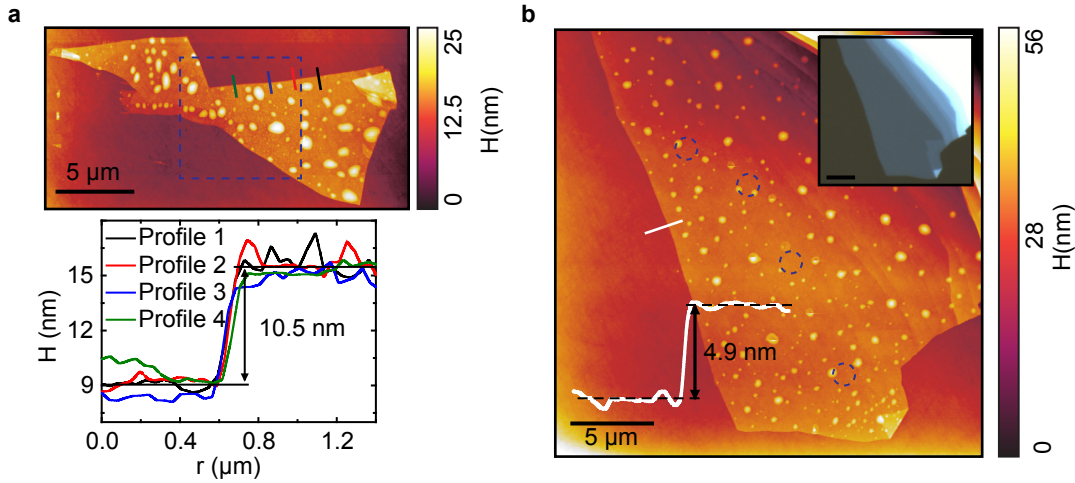

Figure S4: **Absorption coefficient and photooxidation AFM data.** **a**, AFM topography (top) of the  $\text{HfS}_2$  flake presented in figure 3a, main text, after laser exposure of the area marked by the dotted square (see main text). Height profiles across the solid lines are shown in the bottom panel: an average flake thickness of 10.5 nm is reported, corresponding to  $\sim 14$  layers. **b**, AFM topography of the flake used in the photooxidation study shown in figure 2, main text. Dashed circles mark the position where the Raman signal was acquired as a function of time. The flake thickness is 4.9 nm, corresponding to  $\sim 7$  layers. Inset: optical micrograph of the flake immediately after exfoliation on Quartz substrate.

The data regarding the absorption coefficient, presented in figure 4 in the main text and in figure S5, have been acquired on a 10.5 nm thick flake, as shown in Figure S4a. The data shown in figure 2c in the main text have been acquired on a uniform 4.9 nm thick flake, as shown in figure S4b.

## S2.4 Visible wavelength absorption and photoluminescence extended data

Figure S5a shows the absorption coefficient of pristine  $\text{HfS}_2$  as acquired on a thin flake in our experimental setup (see methods). The data are in good agreement with the literature.<sup>6</sup> Transmittance (T), reflectance and absorbance (1-T-R) are shown in figure S5b. Figure S5c shows the photoluminescence (PL) spectra of two representative flakes of bulk  $\text{HfS}_2$  under 473 nm excitation. No strong exciton peak can be seen in proximity of the indirect gap energy whilst the feature at  $\sim 1.7$  eV has been attributed to impurity states in the gap.<sup>7</sup>

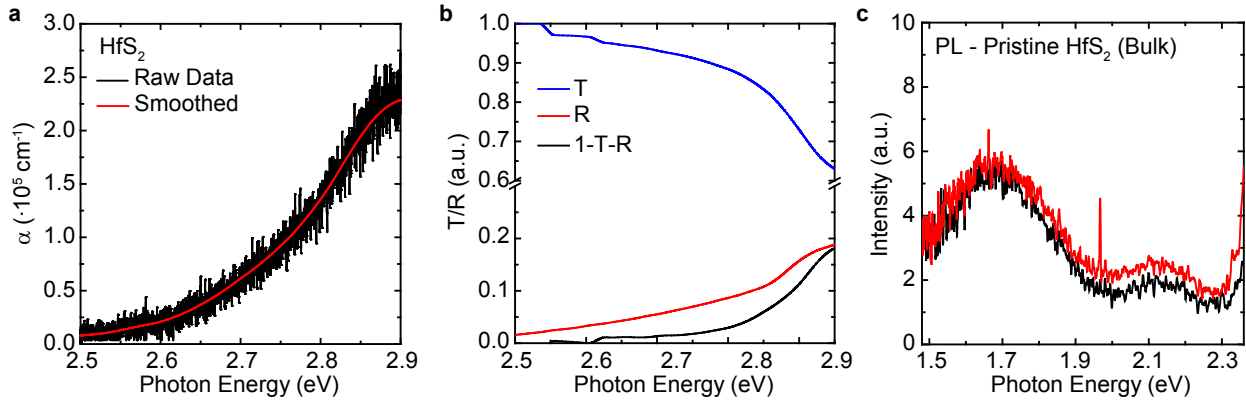

Figure S5: **Absorption coefficient  $\alpha$  of pristine  $\text{HfS}_2$ .** **a**,  $\alpha$  as a function of photon energy in the visible range, as shown in figure 4a, main text. Raw (black) and smoothed (red) data are presented. **b**, Normalised transmittance (T), reflectance (R) and absorbance (1-T-R) as a function of photon energy. **c**, Photoluminescence (PL) spectra of two representative flakes of bulk  $\text{HfS}_2$  under 473 nm excitation.

## S3 First principles calculations

### S3.1 Reactions energy cost

The feasibility of the reaction in equation (S3) has been verified by simulating the crystal structure of the different compounds and calculating the energy cost per reaction, as shown in figure S6 and table S1. The energy cost was calculated as  $E_R = E_{\text{reagents}} - E_{\text{products}}$ .

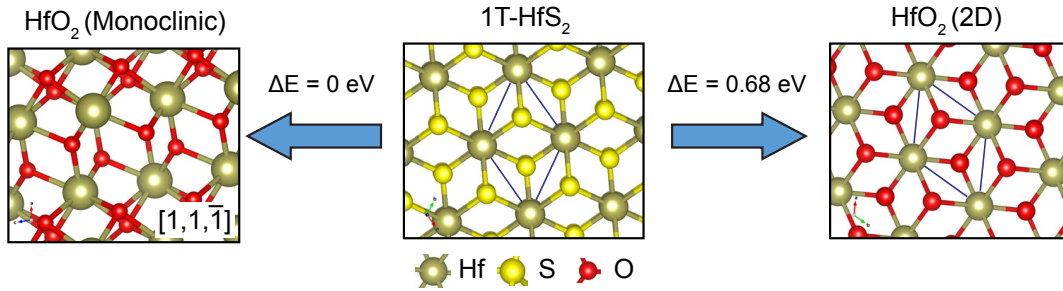

Figure S6: **Reactions energy cost and crystal structures** Simulated crystal structures and energy costs of the proposed reactions. The energy difference  $\Delta E$  is calculated with respect to the formation of monoclinic  $\text{HfO}_2$  ( $E = -11.58$  eV). Unit cell highlighted in blue.

Table S1: Reactions energetics

| Reaction                                                                                                           | Energy cost (eV) | Energy cost (eV) per $\text{HfS}_2$ | $\Delta E$ (eV) <sup>a</sup> per $\text{HfS}_2$ |
|--------------------------------------------------------------------------------------------------------------------|------------------|-------------------------------------|-------------------------------------------------|
| $\text{HfS}_2 + 3 \text{O}_2 \longrightarrow \text{HfO}_2 + 2 \text{SO}_2$ <sup>b</sup>                            | -11.58           | -11.58                              |                                                 |
| $32 \text{HfS}_2 + (32 + 64) \text{O}_2 \longrightarrow \text{Hf}_{32}\text{O}_{64} + 64 \text{SO}_2$ <sup>c</sup> | -370.55          | -11.58                              |                                                 |
| $\text{HfS}_2 + 3 \text{O}_2 \longrightarrow \text{HfO}_2(2\text{D}) + 2 \text{SO}_2$ <sup>f</sup>                 | -10.90           | -10.90                              | 0.68                                            |
| $\text{HfS}_2 + 3 \text{O}_2 \longrightarrow \text{HfO}_2(\text{cubic}) + 2 \text{SO}_2$ <sup>g</sup>              | -11.28           | -11.28                              | 0.30                                            |

<sup>a</sup>Compared to lowest energy reaction; <sup>b</sup> $1 \times 1 \times 1$  Primary unit cell of monoclinic  $\text{HfO}_2$ ;

<sup>c</sup>Large  $2 \times 2 \times 2$  unit cell of monoclinic  $\text{HfO}_2$ ; <sup>f</sup>Energy cost to produce 2D  $\text{HfO}_2$ ; <sup>g</sup>Energy cost to produce cubic  $\text{HfO}_2$ ;

We also considered the possibility of the formation of two-dimensional (2D)  $\text{HfO}_2$ , as opposed to monoclinic 3D  $\text{HfO}_2$ . Such material would be given by the substitution of each S by O in the 2D precursor. However, our calculation shows that the proposed reaction in equation (S3) has an energy cost of  $-10.90$  eV for 2D  $\text{HfO}_2$ , a difference  $\Delta E = 0.68$  eV as compared to 3D (monoclinic)  $\text{HfO}_2$ , which makes the formation of 2D  $\text{HfO}_2$  not favourable.

### S3.2 HfS<sub>2</sub> and HfO<sub>2</sub> band structure

In figure S7a,b we report the calculated band structures of monoclinic HfO<sub>2</sub> and HfS<sub>2</sub>, respectively. In the latter the indirect band gap is  $\sim 1.38$  eV in the  $\Gamma \rightarrow M$  direction, while the direct gap at the  $\Gamma$  point is  $\sim 2.1$  eV. These values are  $\sim 40\%$  off the measured ones<sup>6,8</sup> and in line with other reported DFT calculations.<sup>9</sup> Figure S7c shows the calculated conduction band minimum (CBm) and valence band maximum (VBM) at  $\Gamma$  and in the  $\Gamma \rightarrow M$  direction, as a function of strain. Figure S7d shows the energy difference between the strained and unstrained VBM and CBm.

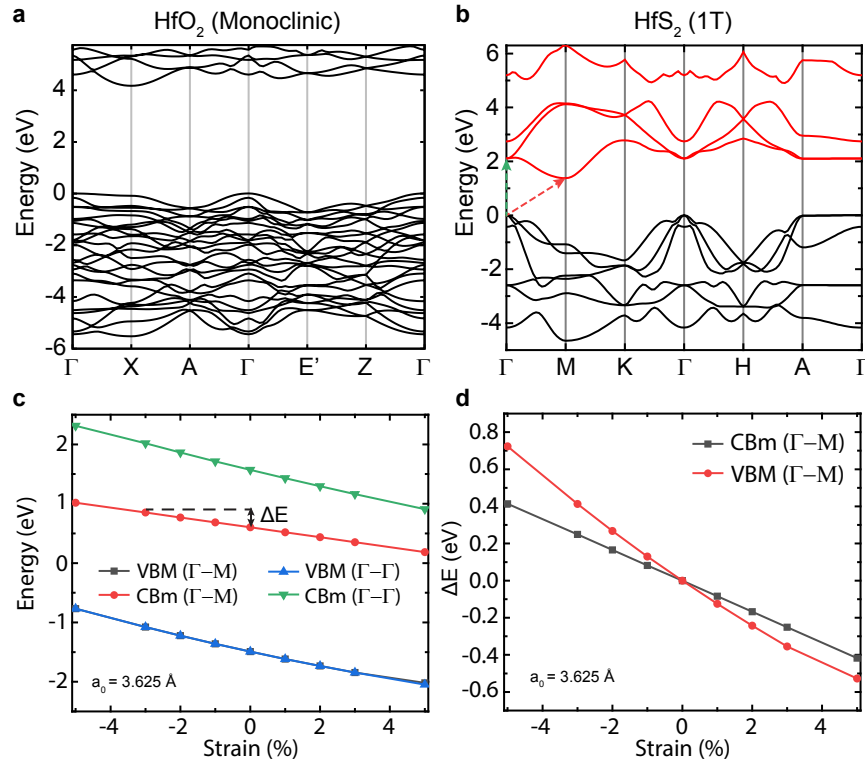

Figure S7: **Band structures of examined compounds.** **a**, Calculated band structure of monoclinic HfO<sub>2</sub>. **b**, Calculated band structure of 1T-HfS<sub>2</sub>. The energy scale is relative to the highest occupied state (0 eV). Black (red) are valence (conduction) states. **c**, Conduction band minimum (CBm) and valence band maximum (VBM) in the  $\Gamma - \Gamma$  direction (red arrow in panel **b**) and in the  $\Gamma - M$  direction (green arrow in panel **b**), as a function of strain. **d**, Difference between the unstrained and strained VBM and CBm in the  $\Gamma - M$  direction.

## S4 Supplementary photoresponse data

### S4.1 Electrical characterization

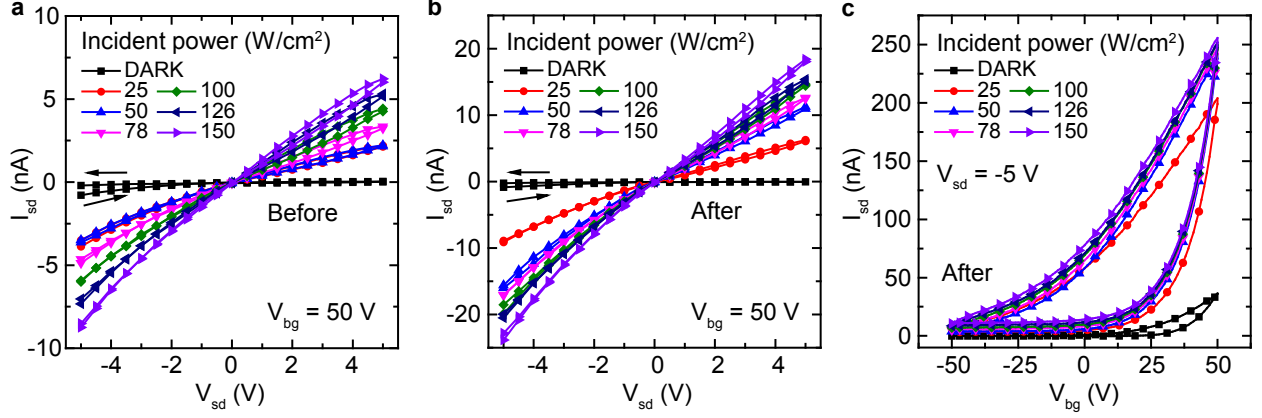

Figure S8: **Electrical characteristic of HfS<sub>2</sub> devices.** **a**, Current-voltage ( $I_{sd}$ - $V_{sd}$ ) characteristic of the device shown in figure 3 main text, before laser-assisted oxidation in the dark and for different incident optical powers ( $\lambda = 473$  nm,  $V_{bg} = +50$  V). **b**, Current-voltage characteristic of the same device after laser-assisted oxidation. **c**, Gate voltage dependence of the photocurrent for the same device, after laser-assisted oxidation,  $V_{sd} = -5$  V.

Figure S8 shows the electrical characterization of the device presented in figure 3 in the main text. Figure S8a shows the current-voltage ( $I_{sd}$ - $V_{sd}$ ) characteristic before the photo-oxidation at different incident optical powers and figure S8b shows the same after the photo-oxidation. Sweeping the  $V_{sd}$  in both direction, no significant hysteresis is observed. In figure S8c we show a gate voltage sweep as a function of incident optical power for the same device. In this case a very large hysteresis is observed, due to the ambient contamination of the device since it is measured in air at room temperature. The observed hysteresis is in agreement with previous results.<sup>10</sup>

### S4.2 Extended photocurrent mapping data

Figure S9a shows the scanning photocurrent microscopy (SPCM) map of the device presented in Figure 4 of the main text, prior to laser-assisted oxidation. Under a bias of  $V_{sd} = \pm 1$  V, the map shows a very small photocurrent generated in the flake, which does not change

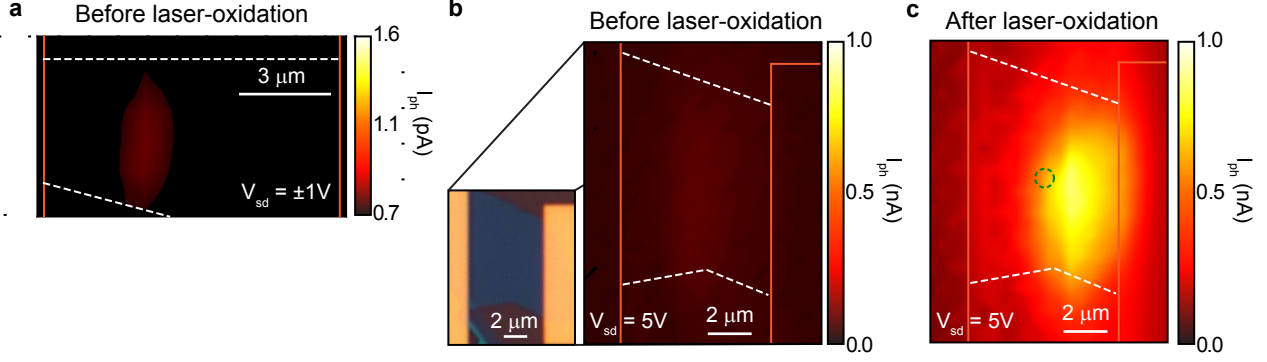

Figure S9: **Extended photocurrent data of  $\text{HfS}_2$  devices.** **a**, Scanning photocurrent microscopy map (SPCM) of the device in Figure 4, main text, before laser assisted oxidation. Under  $V_{sd} = \pm 1 \text{ V}$  only a small photocurrent is observed. For  $V_{sd} = 0 \text{ V}$  no photoresponse could be measured at the sensitivity of our instruments. **b-c**, SPCM maps of another device before and after **(c)** laser assisted oxidation in the centre of the flake (green circle), under  $V_{sd} = 5 \text{ V}$ . Optical micrograph of the device is shown in panel **b**, inset. All SPCM measurements were performed using  $\lambda = 473 \text{ nm}$  at a power  $P = 150 \text{ W/cm}^2$ , as in Figure 4, main text.

117 with the sign of the bias. Therefore we attribute this small contribution to impurities on  
 118 the surface causing local doping of the material. No measurable photocurrent was recorded  
 119 at zero bias. Figure S9b-c show the SPCM maps of another device before and after laser  
 120 assisted oxidation in the centre of the flake, under  $V_{sd} = 5 \text{ V}$ . This device shows the same  
 121 behaviour as the one presented in Figure 3, main text, where a strong localized photocurrent  
 122 is observed after laser-assisted oxidation (green circle). Before laser oxidation no significant  
 123 photocurrent can be observed, as in the previous case.

## 124 S5 Analytical model describing the observed SPCM

### 125 response

126 In this section we develop a simple analytical model which allows to simulate the scanning  
127 photocurrent microscopy (SPCM) results shown in the main text (see figure 4f).

128 In order to describe how local illumination results in a spatial map of the photoresponse  
129 of a device we need to consider the processes of generation, motion and collection of charges.  
130 Starting from the charge continuity equation:

$$\frac{1}{q} \frac{\partial \rho}{\partial t} = G - R - \frac{1}{q} \nabla \cdot \mathbf{j}, \quad (\text{S5})$$

131 where  $\rho$  is the charge density,  $G$  and  $R$  are the generation and recombination rates of the  
132 carriers, respectively and  $\mathbf{j}$  is the current density. Assuming that the average carriers diffusion  
133 length is larger than the laser-spot size we can take  $G$  to be a delta function centred at the  
134 laser excitation point. The recombination rate is equal to  $R_i = -\Delta n_i / \tau_i$ , where  $i = e, h$   
135 indicates the two types of carrier,  $\tau$  is the carrier recombination lifetime and  $\Delta n_i = n_i^t - n_i^d$   
136 is the excited carriers density (difference between the total carrier density  $n_i^t$  and the carrier  
137 density in absence of illumination  $n_i^d$ ). The carrier density can be decomposed into drift and  
138 diffusion terms (we neglect thermoelectric effects):

$$\mathbf{j} = q(n_e \mu_e - n_h \mu_h) \mathbf{E} + q(D_e \nabla n_e - D_h \nabla n_h), \quad (\text{S6})$$

139 where  $\mu_i$  is the mobility,  $\mathbf{E}$  is the electric field across the device and  $D_i = (k_b T \mu_i) / q$  is the  
140 diffusion coefficient at temperature  $T$  with  $k_b \simeq 8.617 \cdot 10^{-5}$  eV/K the Boltzmann constant.  
141 In a junction device or in the presence of a Schottky contact the photocurrent is dominated  
142 by the minority carriers since the drift and diffusion components of the majority carriers will  
143 cancel each other.<sup>11</sup> It is therefore possible to recast equation (S5) in terms of one type of  
144 carrier:

$$\frac{\partial n_e}{\partial t} = -\frac{\Delta n_e}{\tau_e} - \frac{1}{q} \nabla \cdot \mathbf{j}_e. \quad (\text{S7})$$

145 It is important to notice the spatial dependence of  $\Delta n_e$  and  $\mathbf{E}$ . Therefore, for a 1D system,  
 146 equation (S7) takes the form:

$$\frac{\partial n_e}{\partial t} = -\frac{\Delta n_e}{\tau_e} - \mu_e \Delta n_e \frac{\partial E}{\partial x} + \mu_e E \frac{\partial \Delta n_e}{\partial x} + D_e \frac{\partial^2 \Delta n_e}{\partial x^2}. \quad (\text{S8})$$

147 Solving equation (S8) for the steady-state  $\partial n_e / \partial t = 0$ , we obtain:

$$\frac{\partial^2 \Delta n_e}{\partial x^2} + \frac{\mu_e}{D_e} E(x) \frac{\partial \Delta n_e}{\partial x} - \left( \frac{1}{\tau_e D_e} + \frac{\mu_e}{D_e} \frac{\partial E(x)}{\partial x} \right) \Delta n_e = 0. \quad (\text{S9})$$

148 The solution of equation (S9) allows to know  $\Delta n_e$  in each point away from the illumination  
 149 and, therefore, the current can be calculated as:

$$I = -q \int_0^L \left( n_e(x) \mu_e E(x) + D_e \frac{\partial \Delta n_e(x)}{\partial x} \right) dx, \quad (\text{S10})$$

150 where the integral is carried out along the length of the device  $L$ .

151 In order to solve equation (S9) the electric field distribution  $E(x)$  is required. Depending  
 152 on the band structure and the energy profile of photoexcited particles, three type of funnelling  
 153 mechanisms are possible:<sup>12</sup> (1) Type I funnel, where the energy level of electrons continuously  
 154 decreases towards the region of strain, while that of holes increases; (2) Type II funnel, where  
 155 both levels decrease with increasing strain and the exciton binding energy is small (weakly  
 156 bound excitons); (3) Type III funnel, in which the behaviour of the bandgap is the same as  
 157 in type II but in the presence of strongly bound excitons. From the bandgap profiles shown  
 158 in Figure 1b of the main text, and from the absence of a strong excitonic peak in the PL  
 159 spectrum of HfS2 (see figure S5), we conclude that our device is a Type II funnel. In this  
 160 case, due to the weak exciton binding energy, it is possible to replace the potential gradient  
 161 generated by the strain-induced bandgap modulation with an effective electric field. The

simplest model we can adopt is a linear potential from the strained interface ( $x_j$ ) across a region of length  $l_j$ , as depicted schematically in figure S10. The corresponding electric field  $E = -\nabla V$  is given by:

$$E(x) = \begin{cases} -\frac{V_{sd}}{L} \pm \frac{V_0}{l_j}, & x_j - \frac{l_j}{2} \leq x \leq x_j + \frac{l_j}{2} \\ -\frac{V_{sd}}{L}, & \text{otherwise} \end{cases} = \begin{cases} -E_{sd} \pm E_0, & x_j - \frac{l_j}{2} \leq x \leq x_j + \frac{l_j}{2} \\ -E_{sd}, & \text{otherwise} \end{cases}, \quad (\text{S11})$$

which represents the superposition of the applied electric field  $E_{sd}$  and the built-in field due to the strain-induced bandgap modulation  $E_0$ . The plus (minus) sign applies to the left (right) junction, respectively. It is important to notice that the sign of  $E_{sd}$  depends on the applied bias, whilst the sign of  $E_0$  depends on the bandgap gradient and it is fixed at each strain junction. Using equation (S11) in equation (S10) we obtain:

$$\Delta n_e = \begin{cases} \Delta n_e^0 \exp \left\{ -\frac{1}{2} \left( \frac{q}{k_B T} (E_{sd} \pm E_0) + \sqrt{\left( \frac{q}{k_B T} (E_{sd} \pm E_0) \right)^2 + \frac{4}{\tau_e D_e}} \right) |x - x_0| \right\}, & x_j - \frac{l_j}{2} \leq x \leq x_j + \frac{l_j}{2} \\ \Delta n_e^0 \exp \left\{ -\frac{1}{2} \left( \frac{q}{k_B T} E_{sd} + \sqrt{\left( \frac{q}{k_B T} \right)^2 E_{sd}^2 + \frac{4}{\tau_e D_e}} \right) |x - x_0| \right\}, & \text{otherwise} \end{cases}, \quad (\text{S12})$$

where  $\Delta n_e^0$  is the excited carrier density at the injection (illumination) point  $x = x_0$ . We can therefore use equation (S12) and equation (S10) to simulate an SPCM experiment by calculating the total charge injected in the channel at each injection point  $0 \leq x_0 \leq L$ , taking into account that in the oxide region ( $x_{ox} - \frac{l_{ox}}{2} \leq x \leq x_{ox} + \frac{l_{ox}}{2}$ , see figure figure S10)  $\Delta n_e^0 = 0$ , since the bandgap of the oxide is greater than the energy of the impinging photon.

The fit shown in figure 4f, main text, is performed using a value of mobility of  $\mu_e = 2.4 \text{ cm}^2 \text{ V}^{-1} \text{ s}^{-1}$ , which is typical for these devices.<sup>13</sup> The injected charges can be estimated from the photon flux  $\phi = P_{laser}/E_{laser} \simeq 3.5 \cdot 10^{20} \text{ s}^{-1} \text{ cm}^{-2}$  and the internal quantum efficiency  $\eta_i = (I_{ph} E_{laser}/q P_{laser})/(1 - R - T) \simeq 3.0 \cdot 10^{-4}$  (where  $R$  and  $T$  are the reflectivity and transmittance, respectively, as shown in figure S5b), which give a value of injected carriers

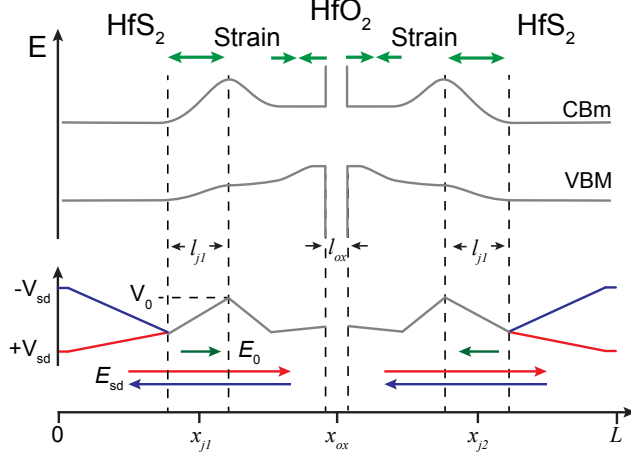

Figure S10: **SPCM model in a strained device.** Schematic band diagram of a strained device with the oxide region at the centre of the channel. There are four strain regions (green arrows), two compressive in the vicinity of the oxide and two tensile far away from it. The simplified potential is shown below for positive ( $+V_{sd}$ ) and negative ( $-V_{sd}$ ) bias.

$\Delta n_e^0 = 1.05 \cdot 10^{17} \text{ s}^{-1} \text{ cm}^{-2}$ . The value of the built-in potential is taken as the difference between the conduction band minimum (CBM) of the strained and unstrained semiconductor, as shown in figure S7c-d, and it is equal to  $V_0 = 0.24 \text{ V}$ . The length of the channel is  $L = 26 \mu\text{m}$  and  $T = 300 \text{ K}$ . The position of the strained junctions can be determined from figure 2, main text:  $l_{j1} = 2.5 \mu\text{m}$  (left) and  $l_{j2} = 2.0 \mu\text{m}$  (right) while the oxide region is  $x_{ox} = 15.0 \mu\text{m}$  and  $l_{ox} = 1.0 \mu\text{m}$ . The carriers lifetime, dominated by non-radiative recombination, is left as a free parameter since, to the best of our knowledge, no experiments are reported in literature with measurement of this value for  $\text{HfS}_2$ . We find that to obtain a good fit and reproduce qualitatively the experimental data we have to assume two different relaxation times for the strained ( $\tau_1$ ) and unstrained ( $\tau_2$ ) regions. We find  $\tau_1 \simeq 1 \cdot 10^{-6} \text{ s}$  and  $\tau_2 \simeq 1 \cdot 10^{-12} \text{ s}$ . The two different values could be explained by a change in electron-hole binding energy due to strain, as previously suggested for different materials.<sup>14</sup>

## S6 Supplementary discussion on PV enhancement using charge funnelling

The main losses in a photovoltaic device are given by two factors: (1) lack of absorption of photons with energy  $E$  smaller than the bandgap of the photoactive material  $E_g$  and (2) dissipation of the kinetic energy of carriers with energy  $E \gg E_g$ . The first process accounts for 23 % of the energy of the sun whilst the second for 33 %.<sup>15</sup> Charge funnelling can tackle both problems. A solution to the first problem has been proposed based on multiple-bandgap tandem solar-cells. With this respect, funnelling offers the ability to continuously tune the bandgap of the active material, effectively realizing a continuous tandem solar cell. The second factor is related to carrier dynamics: after photon absorption carriers are excited in a distribution which mimics the energy distribution of the photons. After a few hundred femtoseconds, carrier-carrier scattering equilibrates this distribution to a population which can be described by a temperature  $T_H$ . In the following tens of picoseconds, carriers lose kinetic energy via phonon emission and relax to a distribution in quasi-equilibrium with the lattice temperature  $T_a$ , a process known as cooling. After this, carriers recombine in different ways to return the system to equilibrium. This dynamics is taken into account in estimating the Shockley-Queisser<sup>16</sup> limit by considering that carriers are completely cooled when extracted at temperature  $T_a$ , for a given bandgap. This calculation gives a theoretical limit of  $\sim 31$  % efficiency for a bandgap of  $E_g \sim 1.3$  eV, under the illumination of a blackbody equivalent to 1 Sun at 5760 K.

As we show in our work, inverse charge funnelling reduces the recombination lifetime of photoexcited carriers from  $10^{-10}$  s to  $10^{-6}$  s. Furthermore, thanks to the modulation of the bandgap and the consequent built-in field in the strain region, the drift velocity is expected to increase. The cooling rate of electrons and holes is inversely proportional to the relaxation time whilst the recombination lifetime is proportional to it.<sup>17</sup> Therefore, the observed reduction of the recombination lifetime can be related to the slowing of the cooling

process, which, together with the increased drift velocity, allow the distribution of hot carriers to be maintained at a temperature  $T_h$ , where  $T_H > T_h > T_a$ . The exploitation of hot-carriers extraction has been largely investigated and the maximum efficiency of a photovoltaic device can be theoretically estimated<sup>15</sup> to be  $\sim 65\%$  at  $E_g \sim 0.5$  eV, under the illumination of a blackbody equivalent to 1 Sun at 5760 K, for a carrier temperature of 3600 K. It is possible to compute such limit for the case of HfS<sub>2</sub>. The estimation of the maximum efficiency of a hot-carrier solar cells relies on a number of assumptions, which should carefully be reviewed in light of what is achievable in a funnel device. One of the main assumptions is that the extraction of carrier is performed with selective contacts which have an energy separation between holes and electrons larger than the bandgap ( $E_{out} > E_g$ , ideally close to the median energy of the hot-electrons distribution) and that extraction is performed in an extremely narrow energy range ( $\Delta E_{out} \ll k_B T$ ). The realization of such effect has been the subject of many studies and attempts to realise hot-carrier extraction using, for example, quantum-confined structures have been reported.<sup>18,19</sup> By taking the above discussion into consideration, it is possible to calculate the current extracted from a hot carrier solar cell:

$$J \cdot E_{out} = q [f_s L(E_g, \text{inf}, T_a, 0) - L(E_g, \text{inf}, T_h, \mu_h) + (1 - f_s) L(E_g, \text{inf}, T_a, 0)], \quad (\text{S13})$$

where  $J$  is the current density,  $f_s = 2.16 \cdot 10^{-5}$  is the angular range of the sun,  $q$  is the charge of the electron,  $\mu_h$  is the chemical potential of the hot electrons and  $L(E_{min}, E_{max}, T, \mu)$  represents the net emitted or absorbed energy flux density integrated over the range  $[E_{min}, E_{max}]$  and it is equal to

$$L(E_{min}, E_{max}, T, \mu) = \frac{2\pi}{h^3 c^2} \int_{E_{min}}^{E_{max}} \frac{E^3}{e^{\frac{E-\mu}{k_B T}} - 1} dE, \quad (\text{S14})$$

where  $h$  is the Planks constant,  $c$  the speed of light and  $k_B$  the Boltzmanns constant. The first term in equation (S13) represents the energy flux density received by the sun, the

239 second term represents the energy flux density absorbed by the solar cell and the third term  
 240 represents the energy flux density emitted by the solar cell into the environment (detailed  
 241 balance limit). From the  $J(V)$  curve it is possible to calculate the extracted power  $P(V) =$   
 242  $V \cdot J$  from the solar cell and, consequently, the maximum efficiency given the three design  
 243 parameters  $E_g, E_{out}$  and  $V$ . Our calculation shows that, for a carrier temperature of 2000 K  
 244 it is possible to achieve a maximum efficiency of  $\sim 45\%$  for a bandgap of 1.96 eV (HfS<sub>2</sub>),  
 245 assuming extraction at the contacts with energy  $\sim 0.2$  eV above the bandgap. Such electron  
 246 temperature has indeed been reported in graphene<sup>20</sup> and the required type of contacts could  
 247 be realised, for example, using heterostructures of 2D materials in order to achieve the  
 248 desired band-alignment.<sup>21</sup> A smaller bandgap can give a higher efficiency, up to 65 %. Such  
 249 requirement can be easily satisfied in a funnel device owing to the ability of TMDs to  
 250 sustain levels of strain up to 11 %<sup>22</sup> and the strong layer-dependent bandgap, which has  
 251 been demonstrated in many 2D materials.<sup>23,24</sup>

## References

- (1) Memming, R. *Semiconductor Electrochemistry*; Wiley, 2008.
- (2) Favron, A.; Gaufres, E.; Fossard, F.; Phaneuf-L'Heureux, A.-L.; Tang, N. Y.-W.; Levesque, P. L.; Loiseau, A.; Leonelli, R.; Francoeur, S.; Martel, R. Photooxidation and quantum confinement effects in exfoliated black phosphorus. *Nat Mater* **2015**, *14*, 826–832.
- (3) Iwasaki, T.; Kuroda, N.; Nishina, Y. Anisotropy of Lattice Dynamical Properties in  $\text{ZrS}_2$  and  $\text{HfS}_2$ . *Journal of the Physical Society of Japan* **1982**, *51*, 2233–2240.
- (4) Cingolani, A.; Lugar, M.; Scamarcio, G.; Lvy, F. The Raman scattering in hafnium disulfide. *Solid State Communications* **1987**, *62*, 121 – 123.
- (5) Roubi, L.; Carlone, C. Resonance Raman spectrum of  $\text{HfS}_2$  and  $\text{ZrS}_2$ . *Phys. Rev. B* **1988**, *37*, 6808–6812.
- (6) Greenaway, D.; Nitsche, R. Preparation and optical properties of group IV-VI chalcogenides having the  $\text{CdI}_2$  structure. *Journal of Physics and Chemistry of Solids* **1965**, *26*, 1445 – 1458.
- (7) Nath, M.; Rao, C. N. R. Nanotubes of Group 4 Metal Disulfides. *Angewandte Chemie International Edition* **2002**, *41*, 3451–3454.
- (8) Traving, M.; Seydel, T.; Kipp, L.; Skibowski, M.; Starrost, F.; Krasovskii, E. E.; Perlov, A.; Schattke, W. Combined photoemission and inverse photoemission study of  $\text{HfS}_2$ . *Phys. Rev. B* **2001**, *63*, 035107.
- (9) Rasmussen, F. A.; Thygesen, K. S. Computational 2D Materials Database: Electronic Structure of Transition-Metal Dichalcogenides and Oxides. *The Journal of Physical Chemistry C* **2015**, *119*, 13169–13183.

- (10) Chae, S. H.; Jin, Y.; Kim, T. S.; Chung, D. S.; Na, H.; Nam, H.; Kim, H.; Perello, D. J.; Jeong, H. Y.; Ly, T. H.; Lee, Y. H. Oxidation Effect in Octahedral Hafnium Disulfide Thin Film. *ACS Nano* **2016**, *10*, 1309–1316.
- (11) Graham, R.; Yu, D. Scanning Photocurrent Microscopy in Semiconductor Nanostructures. *Modern Physics Letters B* **2013**, *27*, 1330018.
- (12) Feng, J.; Qian, X.; Huang, C.-W.; Li, J. Strain-engineered artificial atom as a broad-spectrum solar energy funnel. *Nat Photon* **2012**, *6*, 866–872.
- (13) Xu, K.; Wang, Z.; Wang, F.; Huang, Y.; Wang, F.; Yin, L.; Jiang, C.; He, J. Ultra-sensitive Phototransistors Based on Few-Layered HfS<sub>2</sub>. *Advanced Materials* **2015**, *27*, 7881–7887.
- (14) San-Jose, P.; Parente, V.; Guinea, F.; Roldán, R.; Prada, E. Inverse funnel effect of excitons in strained black phosphorus. *Physical Review X* **2016**, *6*, 1–12.
- (15) Nelson, J. *The Physics of Solar Cells*, 1st ed.; Imperial College Press, 2011; Chapter 10, pp 289–325.
- (16) Shockley, W.; Queisser, H. J. Detailed Balance Limit of Efficiency of p-n Junction Solar Cells. *Journal of Applied Physics* **1961**, *32*, 510–519.
- (17) Sánchez, M. Carrier heating or cooling in semiconductor devices. *Solid-State Electronics* **1973**, *16*, 549 – 557.
- (18) Nozik, A. J. Spectroscopy and hot electron relaxation dynamics in semiconductor quantum wells and quantum dots. *Annual Review of Physical Chemistry* **2001**, *52*, 193–231.
- (19) Watanabe, D.; Kasamatsu, N.; Harada, Y.; Kita, T. Hot-carrier solar cells using low-dimensional quantum structures. *Applied Physics Letters* **2014**, *105*, 171904.
- (20) Johannsen, J. C.; Ulstrup, S.; Cilento, F.; Crepaldi, A.; Zacchigna, M.; Cacho, C.; Turcu, I. C. E.; Springate, E.; Fromm, F.; Raidel, C.; Seyller, T.; Parmigiani, F.;

Grioni, M.; Hofmann, P. Direct View of Hot Carrier Dynamics in Graphene. *Phys. Rev. Lett.* **2013**, *111*, 027403.

(21) Özçelik, V. O.; Azadani, J. G.; Yang, C.; Koester, S. J.; Low, T. Band alignment of two-dimensional semiconductors for designing heterostructures with momentum space matching. *Phys. Rev. B* **2016**, *94*, 035125.

(22) Bertolazzi, S.; Brivio, J.; Kis, A. Stretching and Breaking of Ultrathin MoS<sub>2</sub>. *ACS Nano* **2011**, *5*, 9703–9709.

(23) Xia, F.; Wang, H.; Jia, Y. Rediscovering black phosphorus as an anisotropic layered material for optoelectronics and electronics. *Nature Communications* **2014**, *5*, 4458.

(24) Wang, Q. H.; Kalantar-Zadeh, K.; Kis, A.; Coleman, J. N.; Strano, M. S. Electronics and optoelectronics of two-dimensional transition metal dichalcogenides. *Nat Nano* **2012**, *7*, 699–712.
